# Supplementary material for: Border-Peeling Clustering
Source: arXiv:1612.04869 ancillary file (2019-06-30)
Supplement: Supplementary file 1 [file supplementary_material.pdf]

# Border-Peeling Clustering – Supplementary Material –

## Contents

|                                                        |          |
|--------------------------------------------------------|----------|
| <b>1. Proof of Lemma 1</b>                             | <b>1</b> |
| <b>2. <math>E[b_i^{(0)} x_0]</math> Graph Analysis</b> | <b>2</b> |
| <b>3. Comparison to Spectral Clustering</b>            | <b>3</b> |

## 1. Proof of Lemma 1

**Lemma 1.** Consider a single cluster of  $n$  points in  $\mathbb{R}^1$  distributed uniformly in the interval  $[-1, 1]$  and let  $k = 1$ . Then the expected value of  $b_i^{(0)}$  is given by the following expression:

$$E[b_i^{(0)}|x_i] = \left( \frac{2}{n} + \frac{n(x_i + 1) - 2}{2n} e^{-\frac{n}{2}(x_i + 1)} + \frac{n(1 - x_i) - 2}{2n} e^{-\frac{n}{2}(1 - x_i)} \right) \cdot e^{-1}. \quad (1)$$

**Proof:**

The cluster is uniformly distributed in  $[-1, 1]$ . We model it using  $p_n(x)$ , which describes the density of the cluster at point  $x$ :

$$p_n(x) = \begin{cases} n/2 & |x| \leq 1 \\ 0 & \text{else} \end{cases}.$$

Note that  $\int p_n(x) dx = n$ , thus the expected number of points in the cluster is  $n$ . The probability that there are exactly  $m$  points in the open interval  $(a, b)$  is given according to [1] by the following expression:

$$N_m(a, b) = \frac{\left[\frac{n}{2}(b - a)\right]^m}{m!} e^{-\frac{n}{2}(b - a)}. \quad (2)$$

Consider an arbitrary point  $a \in [-1, 1]$ . Assuming that there is a sample at  $x_i = a$ , we want to calculate  $E[b_i^{(0)}|x_i]$ . For  $k = 1$ ,  $RNN_1^{(0)}(x_i)$  can include at most two points:  $x_i$ 's adjacent left and right neighbors, such that  $b_i^{(0)} = b_i^{left} + b_i^{right}$ , where  $b_i^{left}$  and  $b_i^{right}$  are induced by  $x_i$ 's left and right neighbors, respectively.

We shall begin by calculating  $b_i^{left}$ . Let  $x_j \in [-1, x_i)$  be the left neighbor of  $x_i$  and define  $x'_j$  such that:

$$x'_j = \max\{x_j - (x_i - x_j), -1\} = \max\{2x_j - x_i, -1\}. \quad (3)$$

Since  $k = 1$ , we get that  $x_i \in RNN_1^{(0)}(x_j)$  if and only if both the intervals  $(x_j, x_i)$  and  $(x'_j, x_j)$  are empty. Thus,  $Pr[b_i^{left} = e^{-1}|x_i]$  can be derived as follows:

$$\begin{aligned}
Pr \left[ b_i^{left} = e^{-1} | x_i \right] &= \int_{x_j=-1}^{x_i} N_0(x_j, x_i) \cdot N_0(x'_j, x_j) dx_j = \\
&= \int_{x_j=\frac{x_i-1}{2}}^{x_i} N_0(x_j, x_i) \cdot N_0(2x_j - x_i, x_j) dx_j + \int_{x_j=-1}^{\frac{x_i-1}{2}} N_0(x_j, x_i) \cdot N_0(-1, x_j) dx_j = \\
&= \int_{x_j=\frac{x_i-1}{2}}^{x_i} e^{-\frac{n}{2}(x_i-x_j)} \cdot e^{-\frac{n}{2}(x_j-(2x_j-x_i))} dx_j + \int_{x_j=-1}^{\frac{x_i-1}{2}} e^{-\frac{n}{2}(x_i-x_j)} \cdot e^{-\frac{n}{2}(x_j+1)} dx_j = \\
&= \int_{x_j=\frac{x_i-1}{2}}^{x_i} e^{-n(x_i-x_j)} dx_j + \int_{x_j=-1}^{\frac{x_i-1}{2}} e^{-\frac{n}{2}(x_i+1)} dx_j = \left[ \frac{1}{n} e^{-n(x_i-x_j)} \right]_{\frac{x_i-1}{2}}^{x_i} + \left[ e^{-\frac{n}{2}(x_i+1)} \frac{x_i+1}{2} \right] = \\
&= \frac{1}{n} - \frac{1}{n} e^{-\frac{n}{2}(x_i+1)} + \left[ e^{-\frac{n}{2}(x_i+1)} \frac{x_i+1}{2} \right] = \frac{1}{n} + \frac{n(x_i+1)-2}{2n} e^{-\frac{n}{2}(x_i+1)}.
\end{aligned}$$

A similar calculation for the right side yields

$$Pr \left[ b_i^{right} = e^{-1} | x_i \right] = \frac{1}{n} + \frac{n(1-x_i)-2}{2n} e^{-\frac{n}{2}(1-x_i)}. \quad (4)$$

Thus, since the only possible values for  $b_i^{left}$  and  $b_i^{right}$  are either 0 or  $e^{-1}$ , we conclude that:

$$E \left[ b_i^{(0)} | x_i \right] = \left( \frac{2}{n} + \frac{n(x_i+1)-2}{2n} e^{-\frac{n}{2}(x_i+1)} + \frac{n(1-x_i)-2}{2n} e^{-\frac{n}{2}(1-x_i)} \right) \cdot e^{-1}. \quad (5)$$

■

## 2. $E \left[ b_i^{(0)} | x_0 \right]$ Graph Analysis

In both of the graphs in Figure 2 of the paper, maximal values are achieved in proximity to the borders of the interval. This phenomenon can be explained by the following analysis: consider the case in which  $k = 1$  and a point toward the middle of the cluster,  $x_0$ , that is, a point with many other points to the left of it and many other points to the right of it. Let  $x_r$  be the point right adjacent to  $x_0$  from its right. In general,  $x_0$  competes for the participation in  $NN_k(x_r)$  with another point and wins about half of the times. However, if  $x_0$  is closer to the right (or left) edge of the cluster, then in many cases  $x_0$  will have a right neighbor  $x_r$ , but  $x_r$  has no other neighbor to its right as it is very close to the border, and therefore  $x_0$  does not have to compete with any other point. Hence, the expected value of  $b_i^{(0)}$  is higher for points which are slightly away from the borders.

### 3. Comparison to Spectral Clustering

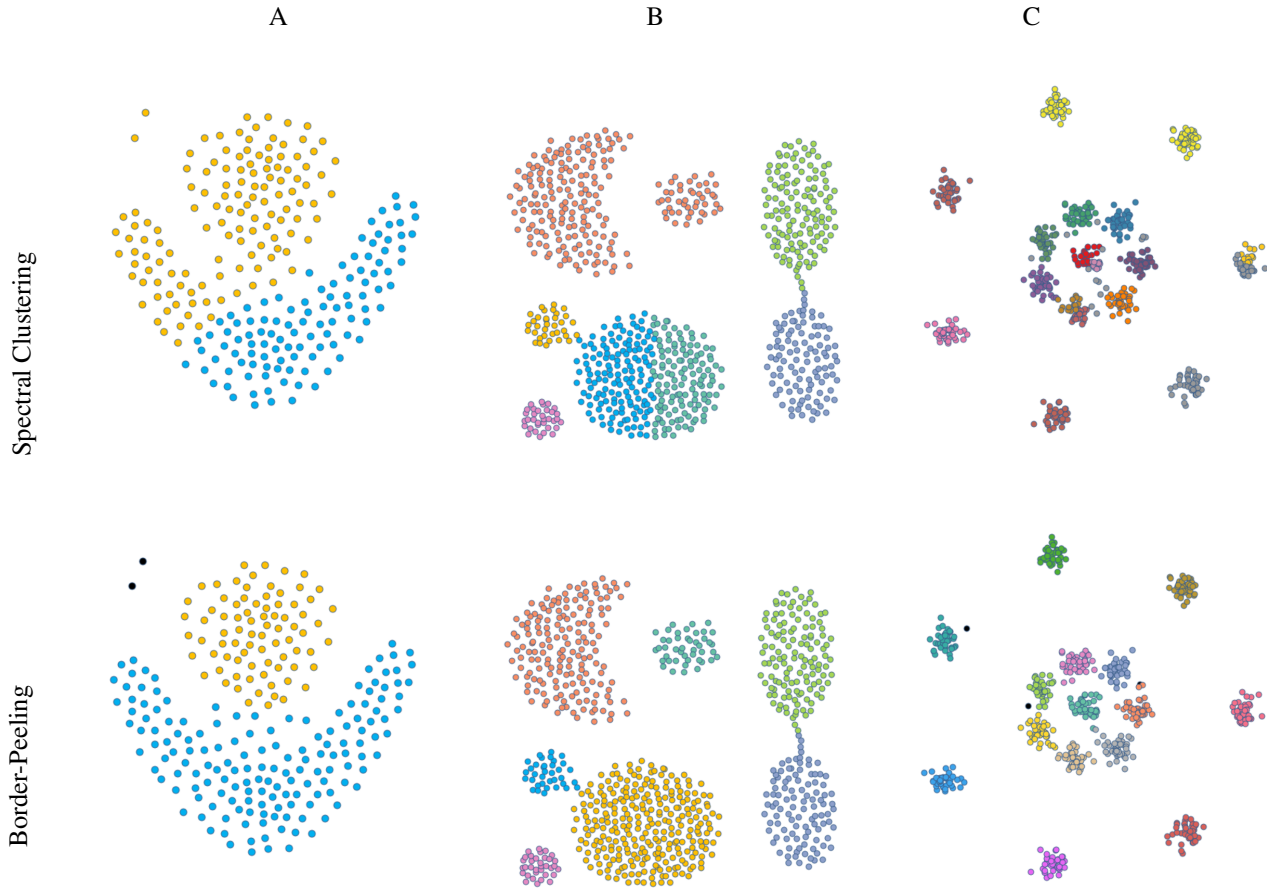

Figure 1: Qualitative comparison of our Border-Peeling technique to the Spectral Clustering [2] technique. Illustrated above are the parametric Spectral Clustering (top row), where the number of clusters is given as input, vs. our non-parametric clustering results (bottom) on three known synthetic examples from the literature (labeled A-C). As the figure demonstrates, Border-Peeling clustering successfully recovered the number of clusters automatically as well as identified the outliers in the synthetic datasets (colored in black), while the Spectral Clustering method failed to identify the correct clusters for data sets A, B and C.

### References

- [1] D. J. Daley and D. Vere-Jones. *An introduction to the theory of point processes: volume I: Elementary Theory and Methods*. Springer Science & Business Media, 2003. 1
- [2] A. Y. Ng, M. I. Jordan, Y. Weiss, et al. On spectral clustering: Analysis and an algorithm. *Advances in neural information processing systems*, 2:849–856, 2002. 3
